# Supplementary material for: Toward Grounded Commonsense Reasoning
Source: arXiv:2306.08651 source file (2024-02-19)
Supplement: Supplementary file 1 [file supplemental.tex]

\documentclass{article}

% === CoRL Template Parameters ===
\usepackage{corl_2023}              % Initial Submission

% ==> Styling & Drafting Macros ==>
\usepackage{amsmath}
\usepackage{amssymb}
\usepackage{booktabs}
\usepackage{enumitem}
\usepackage{graphicx}
\usepackage{hyperref}
\usepackage{pdfx}
\usepackage{subcaption}
\usepackage{xcolor}
\usepackage[export]{adjustbox}
\usepackage[subtle]{savetrees}
\usepackage{enumitem}
\usepackage{listings}
\usepackage[capitalise]{cleveref} % Note --> Must be last import!

% [BREAK GLASS] => USE ONLY AS LAST RESORT
\usepackage{titlesec}
\titlespacing*{\paragraph}{0pt}{0pt}{1em}

% === Custom :: `autoref` Styling ===
%   => Nice Section References, Shorten Figure References...

\def\Snospace~{\S{}}

% === Unified Color Definitions ===
\definecolor[named]{xILIADOrange}{HTML}{FF9B00}
\definecolor[named]{xRefBlue}{HTML}{0055C9}

%   => Colors for Plots / Methods
\definecolor[named]{pOurPink}{HTML}{DE006F}
\definecolor[named]{pAblationLightPink}{HTML}{FF41A0}
\definecolor[named]{pBaselineGray}{HTML}{5A5A5A}
\definecolor[named]{pWeakLightGray}{HTML}{C0C0C0}

%   => Colors for Individual Comments
\definecolor[named]{cMinae}{HTML}{B70101}
\definecolor[named]{cVivek}{HTML}{D027D9}
\definecolor[named]{cSidd}{HTML}{18647E}
\definecolor[named]{cHengyuan}{HTML}{DCF763}

\definecolor[named]{cAnca}{HTML}{FF0000}
\definecolor[named]{cDorsa}{HTML}{FF9D0A}

\definecolor{codegreen}{rgb}{0,0.6,0}
\definecolor{codegray}{rgb}{0.5,0.5,0.5}
\definecolor{codepurple}{rgb}{0.58,0,0.82}
\definecolor{backcolour}{rgb}{0.95,0.95,0.92}

\lstdefinestyle{mystyle}{
    backgroundcolor=\color{backcolour},   
    commentstyle=\color{codepurple},
    keywordstyle=\color{magenta},
    numberstyle=\tiny\color{codegray},
    stringstyle=\color{codegreen},
    basicstyle=\ttfamily\footnotesize,
    breakatwhitespace=false,         
    breaklines=true,                 
    captionpos=b,                    
    keepspaces=true,                 
    numbers=left,                    
    numbersep=5pt,                  
    showspaces=false,                
    showstringspaces=false,
    showtabs=false,                  
    tabsize=2
}
\lstset{style=mystyle}

% === ILIAD Signature ===
\hypersetup{
    colorlinks=true,
    linkcolor=xILIADOrange,
    filecolor=magenta,
    urlcolor=xRefBlue,
    citecolor=xILIADOrange,
}

% === Inline Commenting Macro for each Author --> TODO :: REMOVE ===
%   =>> Usage: \mk{Text to insert...}

% <== Styling & Drafting Macros <==

% === Key Phrase Macros ===
    % [Vivek] => Possible alternatives: TrashTables? SoiledSurfaces?

\begin{document}

\appendix

\section*{Supplementary Material}

% === Individual Appendix Sections ===

\subsection{Data Collection}
\label{appx:data-collection}
\input{sections-appendix/xA_data-collection}

\section{Framework Implementation Details}
\label{appx:evaluation-details}
\input{sections-appendix/xB_evaluation}

\section{Real-World Robot Evaluation}
\label{appx:robot-evaluation}
\input{sections-appendix/xC_robot-evaluation}

\section{VLM Details}
\label{appx:vlm-details}
\input{sections-appendix/xD_vlm}

\section{Personalization Analysis}
\label{appx:personalization}
\input{sections-appendix/xE_personalization}

\section{Prompts \& In-Context Examples for LLM Inference}
\label{appx:prompting-details}
\input{sections-appendix/xF_prompting}

\section{Examples}
\label{appx:examples}
\input{sections-appendix/xG_examples}

% === Bibliography ===
\clearpage
\bibliography{references}

\end{document}
